# Supplementary material for: Optimal Control of the Nonlinear Stochastic Fokker--Planck Equation
Source: arXiv:2406.16512 source file (2025-10-16)
Supplement: Supplementary file 1 [file conditional.tex]

We briefly describe the setup of the control of conditional processes. On a filtered probability space $(\Omega, \F, \bb{F}, \pr)$ equipped with a $d$-dimensional $\bb{F}$-Brownian motion $W = (W_t)_{t \geq 0}$ and a $d$-dimensional $\F_0$-measurable random variable $\xi$, we consider the SDE
\begin{equation}
    \d X_t = \alpha_t \, \d t + \d W_t, \quad X_0 = \xi
\end{equation}
for a $d$-dimensional Brownian motion $W = (W_t)_{t \geq 0}$ and an $\bb{F}$-progressively measurable $\R^d$-valued process $\alpha = (\alpha_t)_{t \geq 0}$ such that $\ev \int_0^T \lvert \alpha_t\rvert^2 \, \d t < \infty$. We call $\mathfrak{a} = (\Omega, \F, \bb{F}, \pr, W, \alpha)$ a \textit{weak control} and denote the space of all such objects by $\bb{A}$. The \textit{cost functional} is given by
\begin{equation}
    J(\mathfrak{a}) = \int_0^T \ev[f(t, X_t, \alpha_t) \vert \tau > t] \, \d t + \ev[g(X_T) \vert \tau > T],
\end{equation}
where $\tau = \inf\{t > 0 \define X_t \notin D\}$ for an open subset $D \subset \R^d$ with $C^1$-boundary and $\bb{E}$ denotes the expectation with respect to $\pr$. We let the \textit{value} $V$ be the infimum of $J(\mathfrak{a})$ over weak controls $\mathfrak{a} \in \bb{A}$. We could consider an extended setup with a drift and diffusion coefficient that depend on time and the location of the diffusion or even its conditional law $\mu_t = \pr(X_t \in \cdot \vert \tau > t)$. The general case introduces additional difficulties, so for the purpose of illustration we stick to this simple setting. 

\begin{assumption} \label{ass:conditional}
Let $f \define [0, T] \times \R^d \times \R^d \to \R$ and $g \define \R^d \to \R$ be measurable and assume there exists $C > 0$ such that
\begin{enumerate}[noitemsep, label = (\roman*)]
    \item for all $(t, x, a)$ we have
    \begin{equation*}
        \lvert f(t, x, a)\rvert + \lvert g(x)\rvert \leq C(1 + \lvert x\rvert^2 + \lvert a\rvert^2);
    \end{equation*}
    \item \label{it:cont_cond} for all $t$ the maps $(x, a) \mapsto f(t, x, a)$ and $x \mapsto g(x)$ are continuous;
    \item \label{it:convex_cond} for all $(t, x)$ the map $a \mapsto f(t, x, a)$ is convex.
\end{enumerate}
\end{assumption}

Our first goal is to prove the equivalence between the weak formulation just introduced and the closed-loop formulation. A \textit{closed-loop control} is a measurable function $a \define [0, \infty) \times \R^d \to \R^d$ such that the SDE
\begin{equation} \label{eq:cond_weak}
    \d X_t = a(t, X_t) \, \d t + \d W_t, \quad X_0 = \xi
\end{equation}
has a weak solution on some filtered probability space $(\Omega, \F, \bb{F}, \pr)$ equipped with a $d$-dimensional $\bb{F}$-Brownian motion $W$ and an $\F_0$-measurable random variable $\xi$, for which $\ev \int_0^T \lvert a(t, X_t)\rvert^2 \, \d t < \infty$. Clearly, SDE \eqref{eq:cond_weak} exhibits uniqueness in law for any measurable function $a \define [0, T] \times \R^d \to \R^d$, so we can introduce the cost functional
\begin{equation}
    J_{\text{cl}}(a) = \int_0^T \ev\bigl[f\bigl(t, X_t, a(t, X_t)\bigr) \big\vert \tau > t\bigr] \, \d t + \ev[g(X_T) \vert \tau > T]
\end{equation}
as well as the associated value $V_{\text{cl}}$, which is simply the infimum of $J_{\text{cl}}(a)$ over all closed-loop controls. It is clear that any closed-loop control $a$ induces a weak control $\mathfrak{a}$ through the assignment $\alpha_t = a(t, X_t)$, so that $V \leq V_{\text{cl}}$. We obtain the reverse inequality through a mimicking argument.

\begin{proposition}
Let Assumption \ref{ass:conditional} be satisfied. For any $K > 0$ and any weak control $\mathfrak{a} = (\Omega, \F, \bb{F}, \pr, W, \alpha)$ with $\lvert \alpha_t\rvert \leq K$ for $\leb \otimes \pr$-a.e.\@ $(t, \omega) \in [0, T] \times \Omega$, there exists a closed-loop control $a$ with corresponding weak solution $(\tilde{\Omega}, \tilde{\F}, \tilde{\bb{F}}, \tilde{\pr}, \tilde{W}, \tilde{\xi}, \tilde{X})$ to SDE \eqref{eq:cond_weak} such that $\pr(X_t \in \cdot \vert \tau > t) = \tilde{\pr}(\tilde{X}_t \in \cdot \vert \tilde{\tau} > t)$ for all $t \in [0, T]$ and $J_{\textup{cl}}(a) \leq J(\mathfrak{a})$, where $\tilde{\tau} = \inf\{t > 0 \define \tilde{X}_t \notin D\}$. In particular, it holds that $V_{\textup{cl}} = V$.
\end{proposition}

\begin{proof}
Let $\mathfrak{a}$ be as in the statement of the theorem and define $X^{\tau}$ by $X^{\tau}_t = X_{\tau \land t}$. The process $X^{\tau}$ satisfies the SDE
\begin{equation*}
    \d X^{\tau}_t = \chi_D(X^{\tau}_t) \alpha_t \, \d t + \chi_D(X^{\tau}_t) \, \d W_t, \quad X^{\tau}_0 = \xi,
\end{equation*}
where $\chi_D \define \R^d \to \{0, 1\}$ is given by $\chi_D(x) = \bf{1}_{x \in D}$. Now, proceeding as in the proof of Theorem 3.7 in \cite{lacker_mfg_controlled_mgale_2015}, using the convexity of $f$ in the control argument guaranteed by Assumption \ref{ass:conditional} \ref{it:convex_cond}, we can find a measurable function $a \define [0, \infty) \times \R^d \to \R^d$ bounded by $K$ such that
\begin{align} \label{eq:meas_sel_cond}
\begin{split}
    \ev\bigl[\chi_D(X^{\tau}_t)\alpha_t \big\vert X^{\tau}_t\bigr] &= \chi_D(X^{\tau}_t)a(t, X^{\tau}_t), \\ \ev\bigl[\chi_D(X^{\tau}_t)f(t, X^{\tau}_t, \alpha_t) \big\vert X^{\tau}_t\bigr] &\geq \chi_D(X^{\tau}_t)f\bigl(t, X^{\tau}_t, a(t, X^{\tau}_t)\bigr)
\end{split}
\end{align}
for $t \in [0, T]$. We may assume that $a(t, x) = 0$ for all $x \in \R^d$ if $t > T$. Then the mimicking theorem by Brunick and Shreve \cite{brunick_mimicking_2013} yields a filtered probability space $(\tilde{\Omega}, \tilde{\F}, \tilde{\bb{F}}, \tilde{\bb{Q}})$ equipped with a $d$-dimensional $\tilde{\bb{F}}$-Brownian motion $\tilde{B}$ and a $d$-dimensional $\tilde{\bb{F}}$-adapted process $\tilde{Y}$ such that
\begin{equation*}
    \d \tilde{Y}_t = \chi_D(\tilde{Y}_t) a(t, \tilde{Y}_t) \, \d t + \chi_D(\tilde{Y}_t) \, \d \tilde{B}_t, \quad \tilde{Y}_0 \sim \L(\xi)
\end{equation*}
and $\L^{\tilde{\pr}}(\tilde{Y}_t) = \L(X^{\tau}_t)$. The latter implies together with \eqref{eq:meas_sel_cond} that
\begin{align} \label{eq:cond_cost_bound}
    J(\mathfrak{a}) &= \int_0^T \frac{\ev\bigl[\chi_D(X^{\tau}_t) f(t, X^{\tau}_t, \alpha_t)\bigr]}{\ev\chi_D(X^{\tau}_t)} \, \d t + \frac{\ev[\chi_D(X^{\tau}_T)g(X^{\tau}_T)]}{\ev\chi_D(X^{\tau}_T)} \notag \\
    &\geq \int_0^T \frac{\ev\bigl[\chi_D(X^{\tau}_t) f\bigl(t, X^{\tau}_t, a(t, X^{\tau}_t)\bigr)\bigr]}{\ev\chi_D(X^{\tau}_t)} \, \d t + \frac{\ev[\chi_D(X^{\tau}_T)g(X^{\tau}_T)]}{\ev\chi_D(X^{\tau}_T)} \notag \\
    &= \int_0^T \frac{\ev^{\tilde{\bb{Q}}}\bigl[\chi_D(\tilde{Y}_t) f\bigl(t, \tilde{Y}_t, a(t, \tilde{Y}_t)\bigr)\bigr]}{\ev^{\tilde{\bb{Q}}}\chi_D(\tilde{Y}_t)} \, \d t + \frac{\ev^{\tilde{\bb{Q}}}[\chi_D(\tilde{Y}_T)g(\tilde{Y}_T)]}{\ev^{\tilde{\bb{Q}}}\chi_D(\tilde{Y}_T)}.
\end{align}

We wish to extend $\tilde{Y}$ to a solution of SDE \eqref{eq:cond_weak}. For that, we perform the change of measure 
\begin{equation*}
    \frac{\d \tilde{\pr}}{\d \tilde{\bb{Q}}}\bigg\vert_{\tilde{\F}} = \cal{E}\biggl(\int_0^{\cdot} (1 - \chi_D(\tilde{Y}_t)) a(t, \tilde{X}_t) \cdot \d \tilde{B}_t\biggr)_{\infty},
\end{equation*}
where the process $\tilde{X} = (\tilde{X}_t)_{t \geq 0}$ is given by $\tilde{X}_t = \tilde{Y}_t$ if $t < \tilde{\tau}$ and $\tilde{X}_t = \tilde{Y}_{\tilde{\tau}} + \tilde{B}_t - \tilde{B}_{\tilde{\tau}}$ otherwise. By Girsanov's theorem, the process $\tilde{W} = (\tilde{W}_t)_{t \geq 0}$ defined by $\tilde{W}_t = \tilde{B}_t - \int_0^t (1 - \chi_D(\tilde{Y}_s)) a(s, \tilde{X}_s) \, \d s$ is a $d$-dimensional $\tilde{\bb{F}}$-Brownian motion under $\tilde{\pr}$. Moreover, we claim that $\tilde{X}$ is a weak solution to SDE \eqref{eq:cond_weak} on $(\tilde{\Omega}, \tilde{\F}, \tilde{\bb{F}}, \tilde{\pr})$ with Brownian motion $\tilde{W}$ and initial condition $\tilde{\xi}$. Indeed, $\tilde{X}$ clearly satisfies SDE \eqref{eq:cond_weak} on $[0, \tilde{\tau})$, since $\tilde{W} = \tilde{B}$ on $[0, \tilde{\tau})$ and $\tilde{Y}$ solves SDE \eqref{eq:cond_weak} on $[0, \tilde{\tau})$ with Brownian motion $\tilde{B}$. Next, assume that $t > \tilde{\tau}$. Then, it holds that
\begin{align*}
    \tilde{X}_t &= \tilde{Y}_{\tilde{\tau}} + \tilde{B}_t - \tilde{B}_{\tilde{\tau}} \\
    &= \tilde{Y}_0 + \int_0^{\tilde{\tau}} \chi_D(\tilde{Y}_s) a(s, \tilde{Y}_s) \, \d s + \tilde{B}_{\tilde{\tau}}  + \tilde{B}_t - \tilde{B}_{\tilde{\tau}} \\
    &= \tilde{Y}_0 + \int_0^{\tilde{\tau}} a(s, \tilde{X}_s) \, \d s + \int_0^t (1 - \chi_D(\tilde{Y}_s)) a(s, \tilde{X}_s) \, \d s + \tilde{W}_t \\
    &= \tilde{Y}_0 + \int_0^t a(s, \tilde{X}_s) \, \d s + \tilde{W}_t,
\end{align*}
so $\tilde{X}$ also solves SDE \eqref{eq:cond_weak} for $t > \tilde{\tau}$. Moreover, in view of Equation \eqref{eq:cond_cost_bound} we have that
\begin{align*}
    J(\mathfrak{a}) &\geq \int_0^T \frac{\ev^{\tilde{\pr}}\bigl[\chi_D(\tilde{X}_t) f\bigl(t, \tilde{X}_t, a(t, \tilde{X}_t)\bigr)\bigr]}{\ev^{\tilde{\pr}}\chi_D(\tilde{X}_t)} \, \d t + \frac{\ev^{\tilde{\pr}}[\chi_D(\tilde{X}_T)g(\tilde{X}_T)]}{\ev^{\tilde{\pr}}\chi_D(\tilde{X}_T)} = J_{\text{cl}}(a),
\end{align*}
where we used that $\tilde{\bb{Q}}$ and $\tilde{\pr}$ coincide on $\tilde{\F}_{\tilde{\tau} \land T}$. It remains to show that the conditional laws of $X_t$ and $\tilde{X}_t$ coincide. This follows from $\L^{\tilde{\pr}}(\tilde{Y}_t) = \L(X^{\tau}_t)$, since for $t \in [0, T]$ we have
\begin{align*}
    \pr(X_t \in A \vert \tau > t) &= \frac{\ev[\bf{1}_{\tau > t} \bf{1}_{X_t \in A}]}{\ev\bf{1}_{\tau > t}} = \frac{\ev[\chi_D(X^{\tau}_t )\bf{1}_{X^{\tau}_t \in A}]}{\ev\chi_D(X^{\tau}_t)} = \frac{\ev^{\tilde{\bb{Q}}}[\chi_D(\tilde{Y}_t )\bf{1}_{\tilde{Y}_t \in A}]}{\ev^{\tilde{\bb{Q}}}\chi_D(\tilde{Y}_t)} \\
    &= \frac{\ev^{\tilde{\pr}}[\chi_D(\tilde{X}^{\tilde{\tau}}_t )\bf{1}_{\tilde{X}^{\tilde{\tau}}_t \in A}]}{\ev^{\tilde{\pr}}\chi_D(\tilde{X}^{\tilde{\tau}}_t)} = \tilde{\pr}(\tilde{X}_t \in A \vert \tilde{\tau} > t),
\end{align*}
where $\tilde{\tau} = \inf\{t > 0 \define \tilde{Y} \notin D\} = \inf\{t > 0 \define \tilde{X} \notin D\}$.

The last statement follows from a simple limit procedure. Let us choose a sequence of weak controls $\mathfrak{a}^k = (\Omega^k, \F^k, \bb{F}^k, W^k, \alpha^k)$ such that $\lvert \alpha_t^k\rvert \leq k$ and $\lim_{k \to \infty} J(\mathfrak{a}^k) = V$. Such a sequence exists owing to the continuity condition from Assumption \ref{ass:conditional} \ref{it:cont_cond}. According to what we proved above, for each $k \geq 1$, there exists a closed-loop control $a^k$ such that $J_{\text{cl}}(a^k) = J(\mathfrak{a}^k)$. Consequently, we get
\begin{equation*}
    V_{\text{cl}} \leq \limsup_{k \to \infty} J_{\text{cl}}(a^k) = \limsup_{k \to \infty} J(\mathfrak{a}^k) = V,
\end{equation*}
which concludes the proof.
\end{proof}

% Let us now consider the regularised framework, where the absorption is replaced by killing at a state-dependent rate. We let $\lambda \define \R^d \to [0, \infty)$ be a Lipschitz continuous function such that $\lambda(x) = 0$ if $x$ lies in the closure of $D$ and $\lambda(x) > 0$ otherwise. Then let $(X, \Lambda) = (X_t, \Lambda_t)_{t \geq 0}$ solve the SDE
% \begin{equation} \label{eq:conditional_sde}
%     \d X_t = b(t, X_t, \mu_t) \, \d t + \sigma(t, X_t, \mu_t) \, \d W_t, \quad \Lambda_t = \lambda(t, X_t, \mu_t) \, \d t
% \end{equation}
% with initial condition $X_0 = \xi$ and $\Lambda_0 = 0$. The data $W$, and $\xi$ are as in the beginning of the section and $\mu_t = \pr(X_t \in \cdot \vert \theta > \Lambda_t)$, where $\theta$ is an exponential random variable independent of $W$ and $\xi$. Without discussion existence and uniqueness of the \textit{conditional SDE} \eqref{eq:conditional_sde}, we would like to propose a particle representation with matching marginal distributions. 

% We need some preparation. 
